# Supplementary material for: SegSplat: Feed-forward Gaussian Splatting and Open-Set Semantic Segmentation
Source: arXiv:2511.18386 source file (2025-11-23)
Supplement: Supplementary file 1 [file 6_appendix.tex]

\section{Appendix}
\label{sec:appendix}

\subsection{SegSplat Segmentation Results on RE10k}

We provide additional visualizations of the segmentation masks produced by SegSplat on the RE10k dataset~\cite{realestate10k} shown in Figure~\ref{fig:re10k_segsplat_segmentations}.
For each scene, we prompt for prominent objects found in RE10k, such as \emph{"chair"}, \emph{"desk"}, or \emph{"couch"}. We observe that without any scene-specific training, SegSplat is able to produce accurate segmentation masks for most text prompts.
\begin{figure}[htp]
  \centering
  \includegraphics[width=0.25\linewidth]{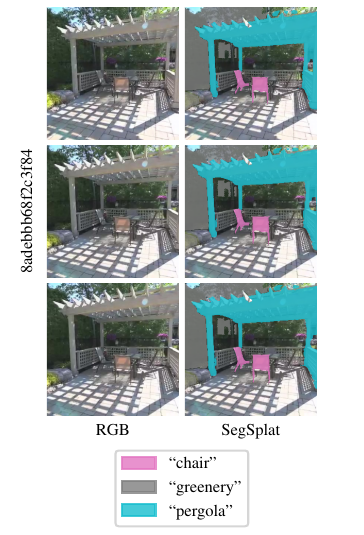}%
  \includegraphics[width=0.25\linewidth]{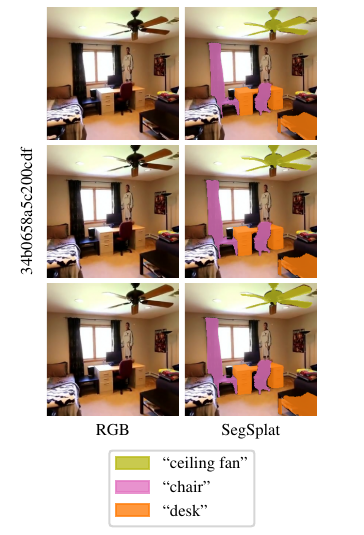}%
  \includegraphics[width=0.25\linewidth]{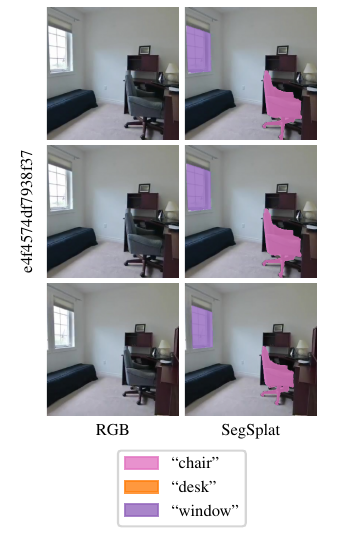}%
  \includegraphics[width=0.25\linewidth]{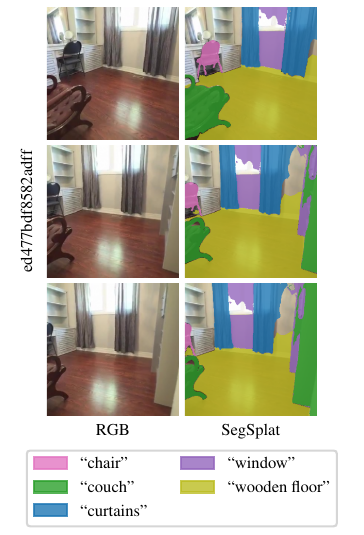}%
  \caption{A visualization of the masks produced by SegSplat on the RE10k dataset~\cite{realestate10k} using multiple text queries, as noted below each plot. We show results for four scenes and three different novel views in each scene.}
  \label{fig:re10k_segsplat_segmentations}
  \vspace{-5mm}
\end{figure}

\subsection{SegSplat vs. LangSplat Feature Comparison}

We show a side-by-side comparison of SegSplat and LangSplat on the 3D-OVS dataset~\cite{liu2023weakly} in Figure~\ref{fig:3d_ovs_side_by_side_scene_comparison}. In general, we observe that SegSplat produces more accurate and less noisy semantic features compared to LangSplat, reflected in the IoU scores shown in Table~\ref{table:iou_comparison}.

\begin{figure}[htp]
  \centering
  \subfloat[SegSplat]{
    \includegraphics[width=0.9\linewidth]{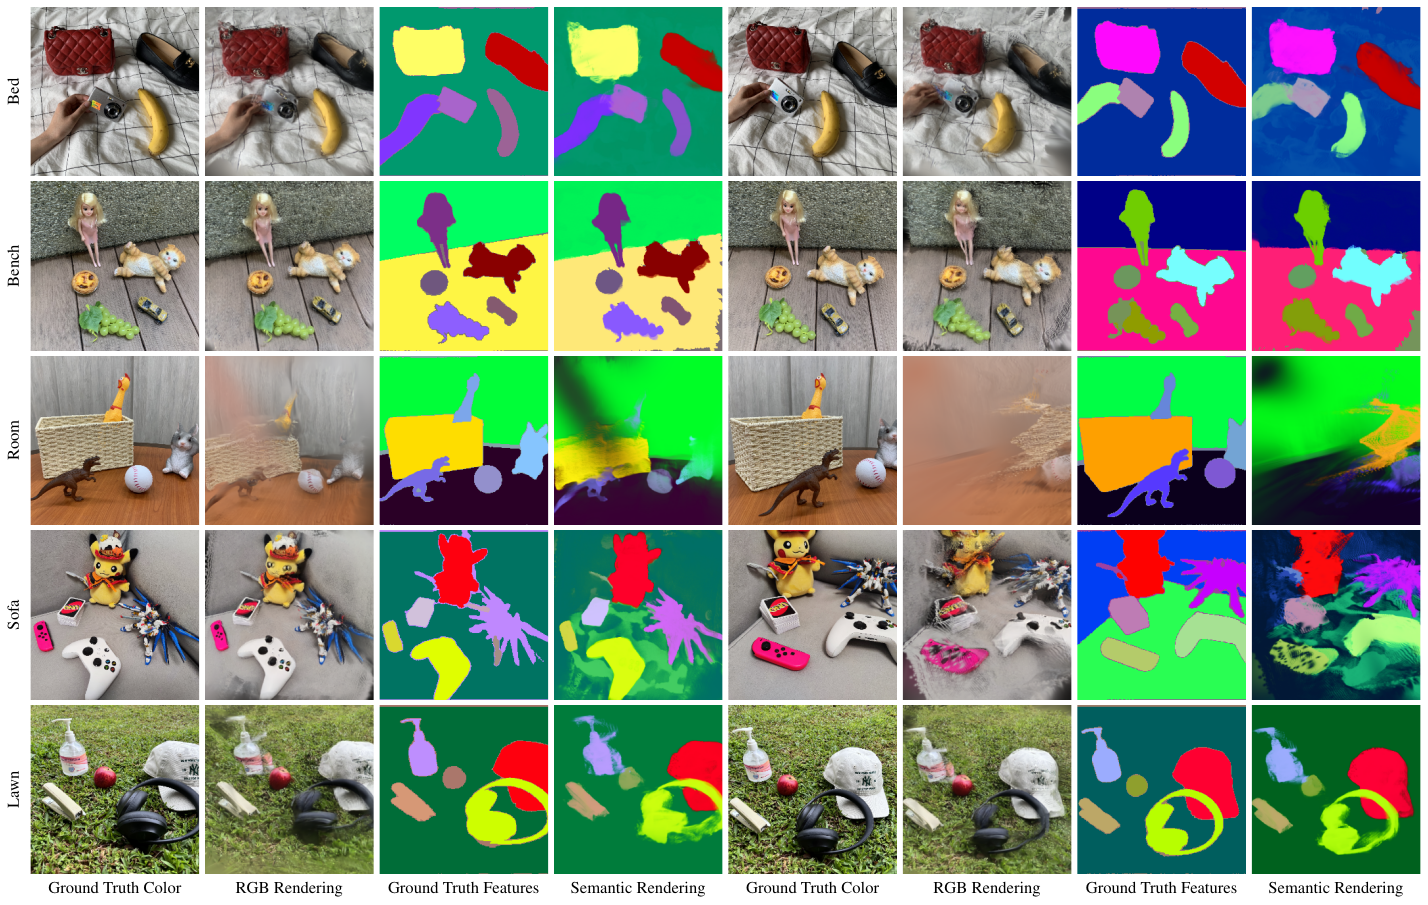}
    \label{fig:segsplat}
  }\\[1mm]
  \subfloat[LangSplat]{
    \includegraphics[width=0.9\linewidth]{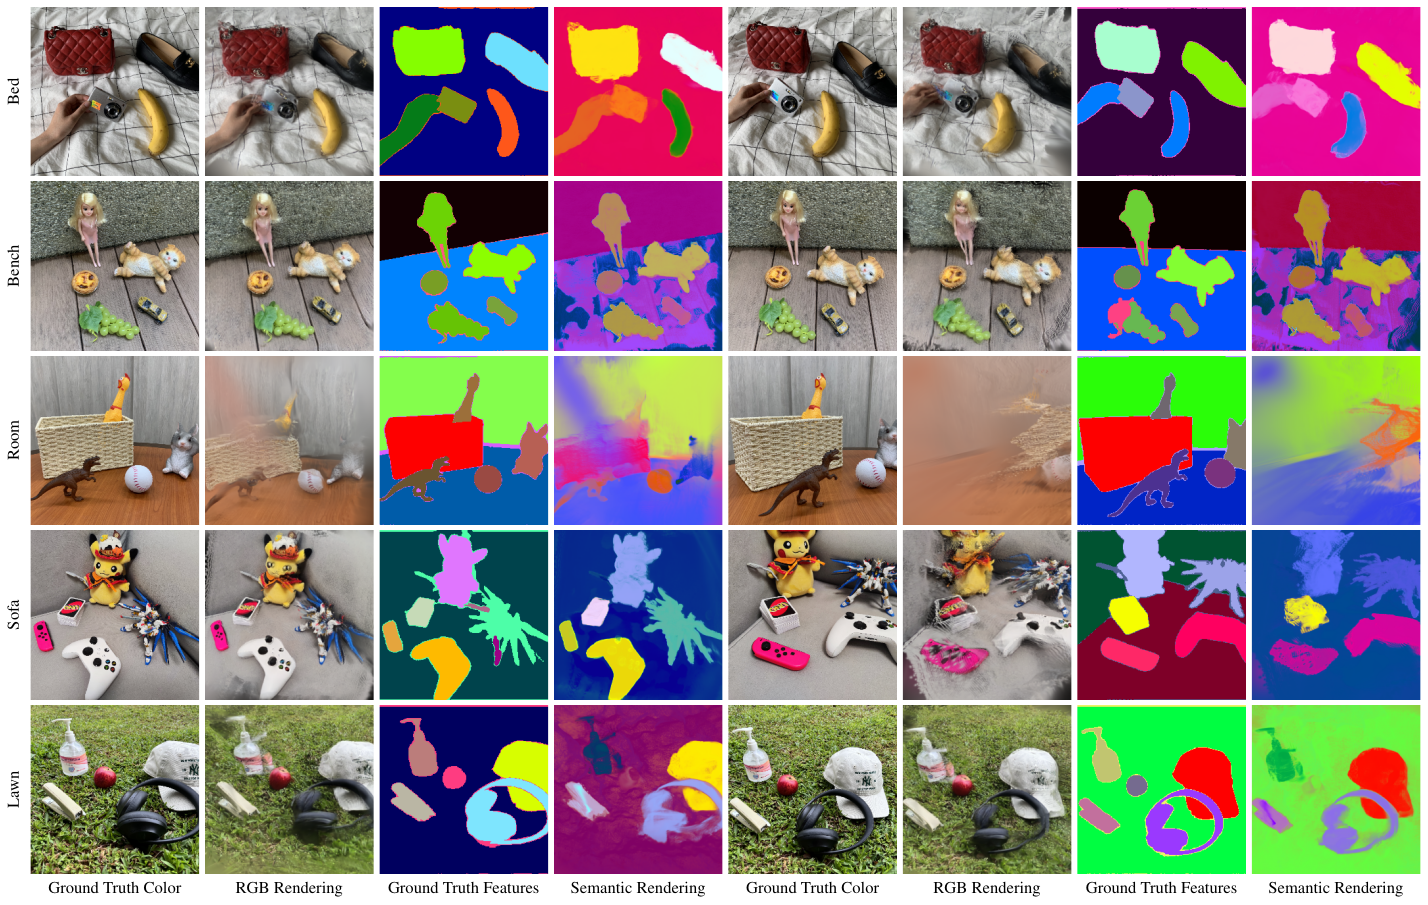}
    \label{fig:langsplat}
  }
  \caption{
    Comparison of predicted and ground truth (GT) color and semantic maps for novel views rendered by SegSplat (a) and LangSplat (b) on the 3D-OVS dataset~\cite{liu2023weakly}.
    Semantic maps are visualized using PCA. Ground truth semantic features are obtained by applying SAM+CLIP to the corresponding GT novel view images.
    For LangSplat, we first decode the rendered semantic features using the learned autoencoder before applying PCA.
    Each group of four columns shows: GT RGB image, rendered RGB, GT semantics, and rendered semantics, repeated for two novel views.
    Our method (a) produces more accurate and less noisy semantic features compared to (b).
  }
  \label{fig:3d_ovs_side_by_side_scene_comparison}
  \vspace{-5mm}
\end{figure}

\subsection{K-Means Clustering Optimization}

In the main paper, we proposed using a heuristic to compute the number of clusters $M$ for K-Means during the semantic feature bank construction. We follow the formula $M = \lambda N_\text{total} / K$ where $N_\text{total}$ is the total number of masks from all $K$ input views. This heuristic aims to accommodate varying object visibility across views, e.g., in the case where more objects identified by SAM are visible in one view than another. Figure \ref{fig:3d_ovs_kmeans_iou_comparison} shows the IoU scores for different values of $\lambda$ on the 3D-OVS dataset. We observe that $\lambda=1.2$ yields the best performance and use this value for all of our experiments.
Let us also note that above $1.2$, the results seem to be stable and close to the no-clustering case.

\begin{figure}[htp]
  \centering
  \includegraphics[width=0.9\linewidth]{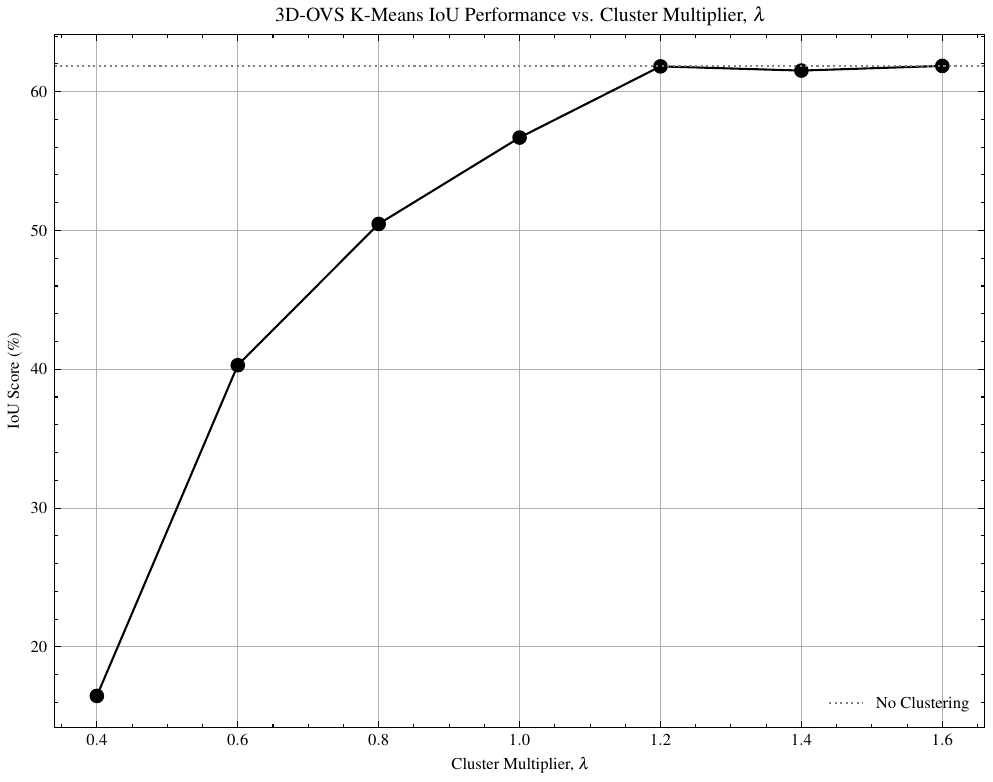}
  \caption{
    We perform a search on the 3D-On the 3D-OVS dataset for the optimal $\lambda$ used to compute the number of clusters for each input (Section \ref{sec:experiments}).
    We observe that $\lambda=1.2$ yields the best performance while reducing the length of the feature encoding by $40 \%$ and producing IoU results nearly identical to those obtained with K-Means clustering disabled.
  }
  \label{fig:3d_ovs_kmeans_iou_comparison}
\end{figure}
